# Supplementary material for: Chain-Length-Dependent Partitioning of 1-Alkanols in Raft-Like Lipid Membranes
Source: arXiv:2601.18095 source file (2026-01-26)
Supplement: Supplementary file 1 [file alkanol_mem_SupplementaryInformation_jchemphys.pdf]

# Supplementary Information

## Chain-Length-Dependent Partitioning of 1-Alkanols in Raft-Like Lipid Membranes

Anirban Polley

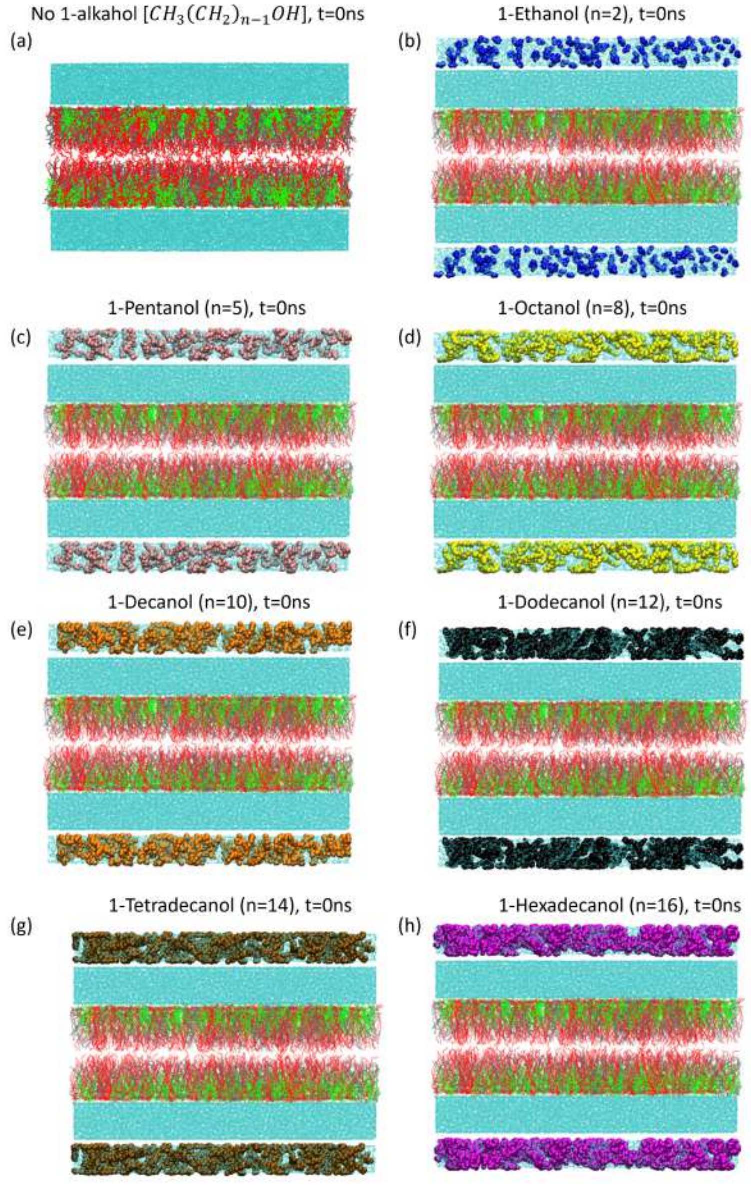


**Fig. S1** Snapshot of initial configuration of the symmetric bilayer membranes comprising DOPC (grey), DPPC (red), Chol (green), water (cyan) (a) without 1-alkanol, and the composite membrane having 1-alkanol with (b) 1-Ethanol (blue), (c) 1-Pentanol (pink), (d) 1-Octanol (yellow), (e) 1-Decanol (orange), (f) 1-Dodecanol (black), (g) 1-Tetradecanol (dark orange) and (h) 1-Hexadecanol (purple) are shown respectively.

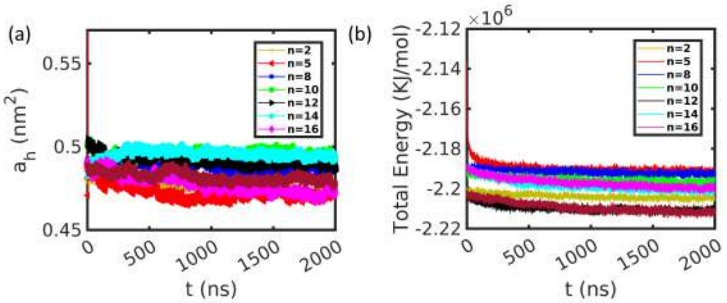


**Fig. S2** The time evolution of area of the lipid and total energy of composite membrane without and with 1-alkanols with varying chain length $n$, respectively indicating the equilibration of the simulations.

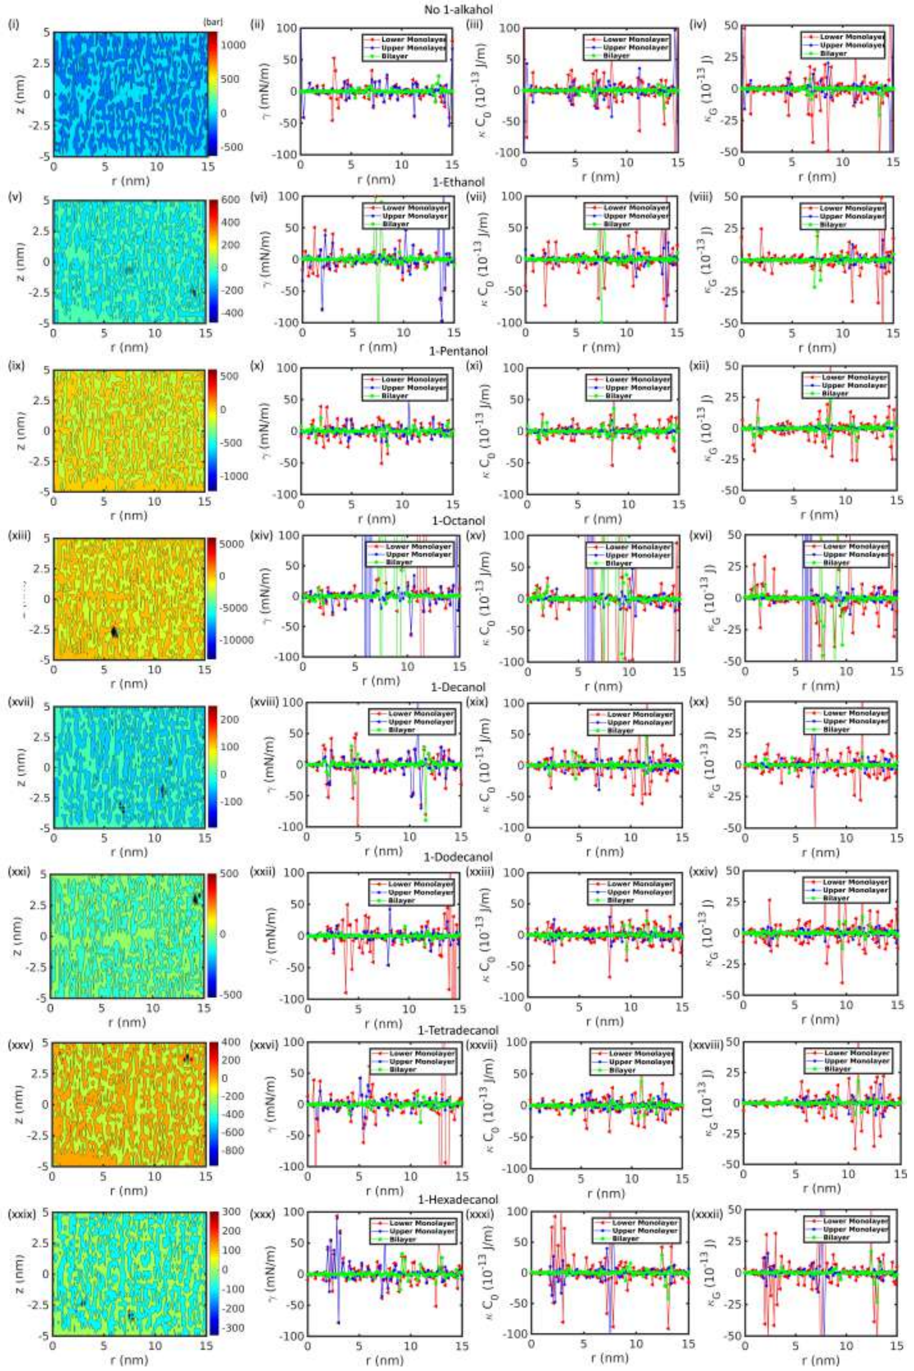


**Fig. S3** The pressure profile, surface tension $\gamma$, product of bending rigidity and spontaneous curvature $\kappa C_0$ and elastic modulus of Gaussian curvature $\kappa_G$ of the composite membrane wiout and with 1-alkanols with varying chain length $n$.

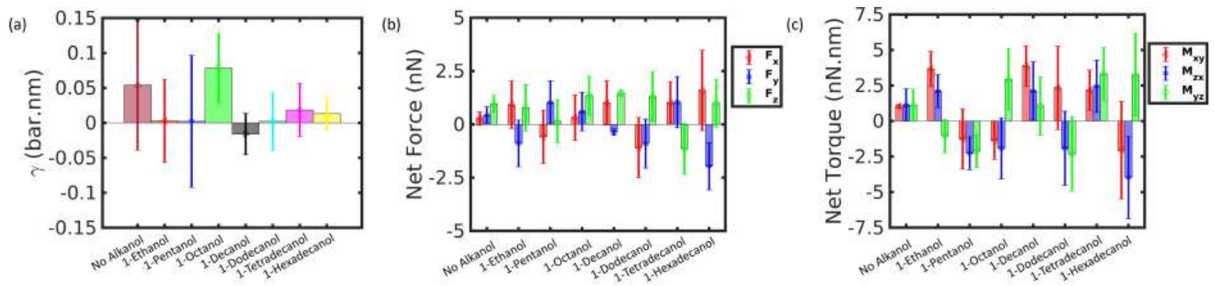


**Fig. S4** Average surface tension $\gamma$, net force components ($F_x$, $F_y$, and $F_z$) and net torque components ($M_{xy}$, $M_{yz}$ and $M_{zx}$) of the composite membrane wiout and with 1-alkanols with varying chain length $n$.

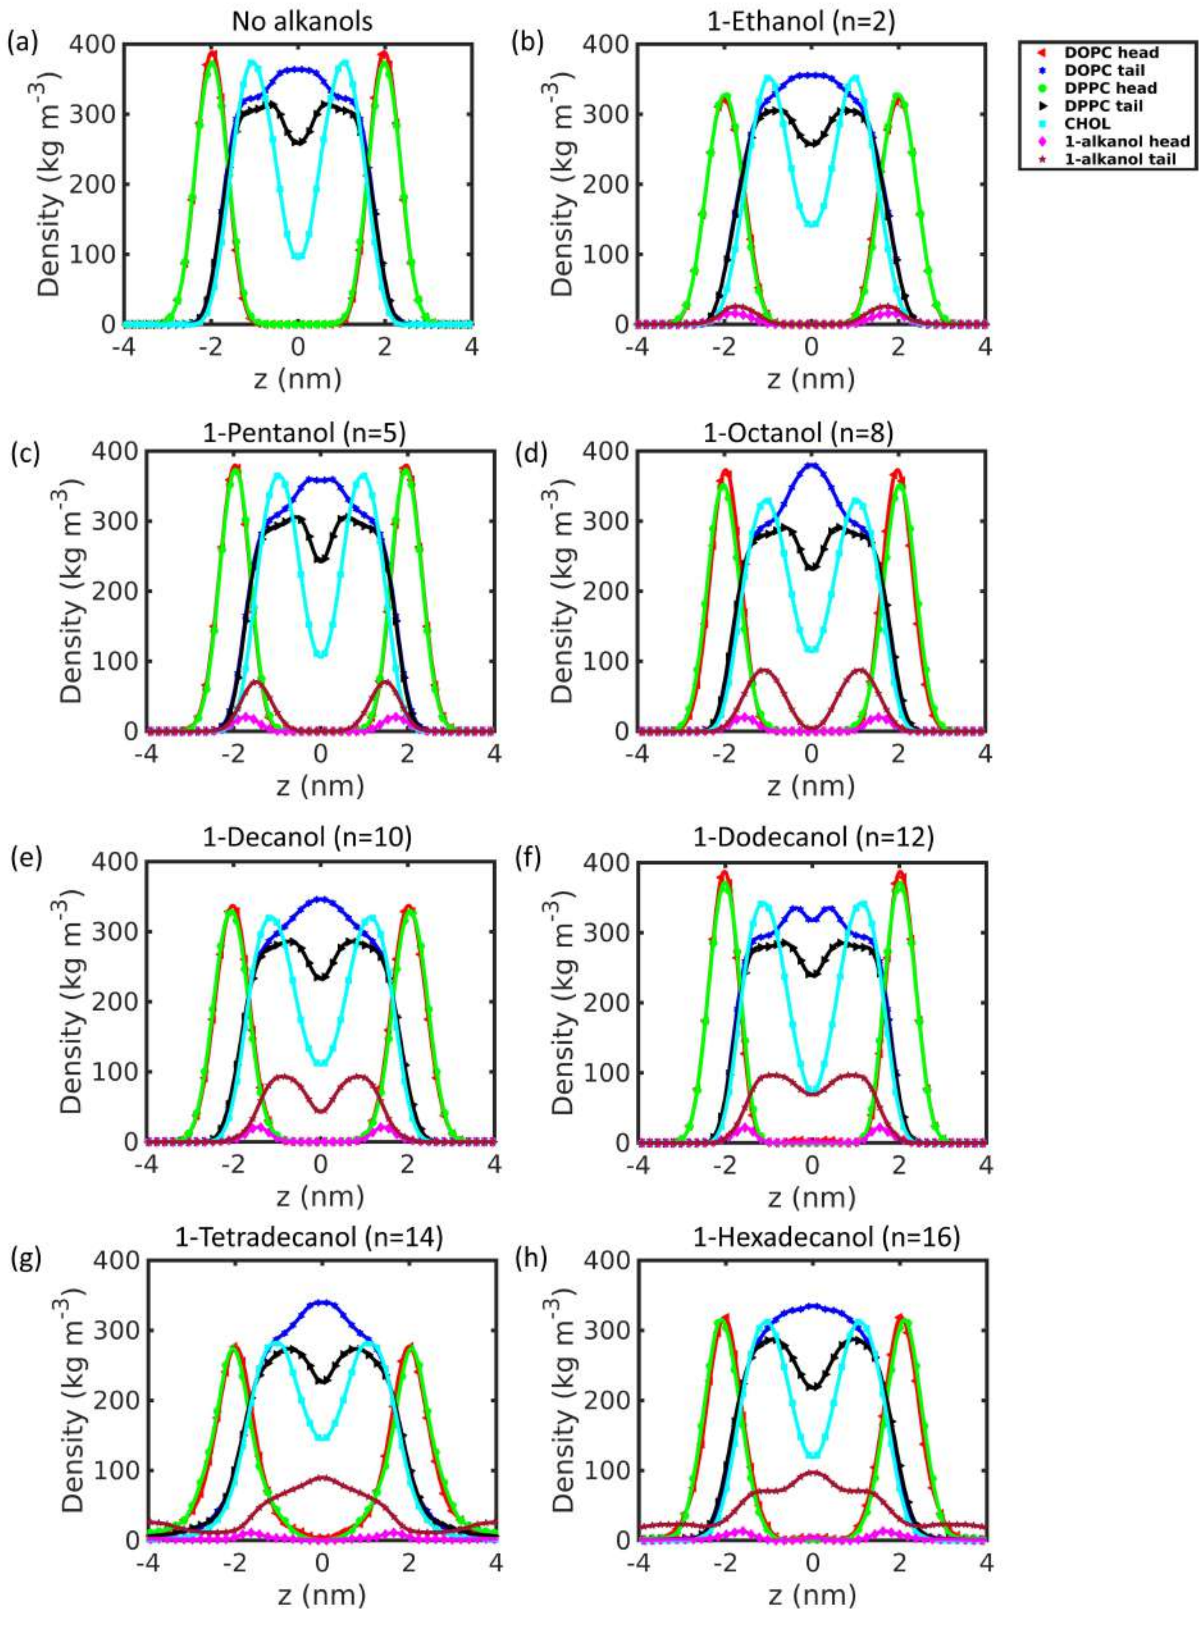


**Fig. S5** Density profile of the headgroup and tail of DOPC, DPPC lipids, Chol, and the headgroup and tail of 1-alkanols of composite membrane without and with 1-alkanols with varying chain length $n = 2$, 5, 8, 10, 12, 14 and 16, respectively.

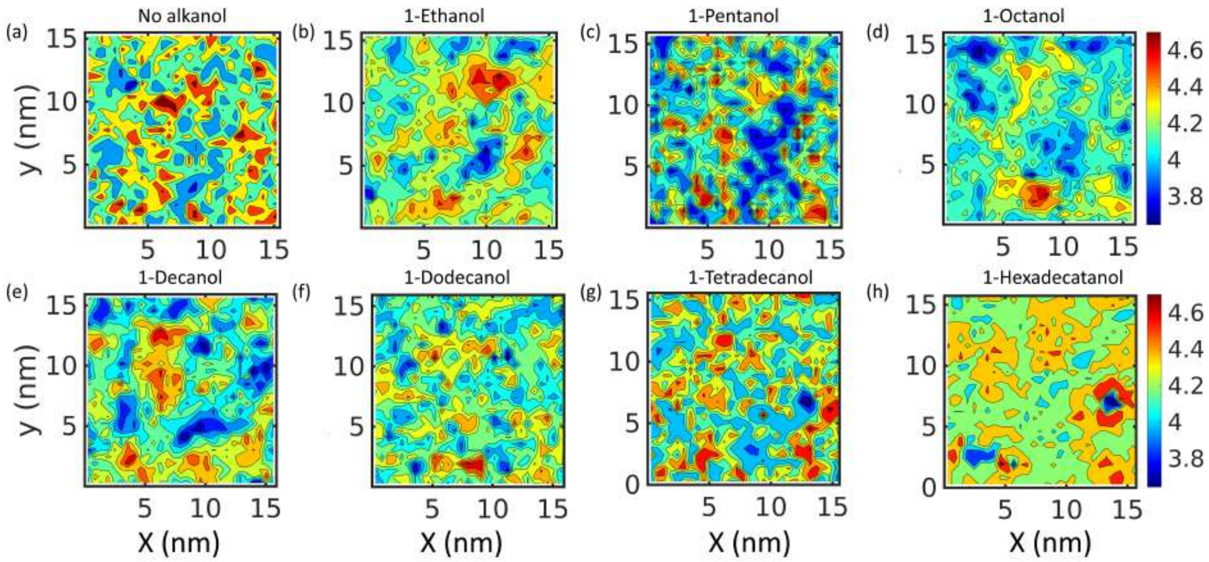


**Fig. S6** Spatial heterogeneity of the thickness of the composite membrane without and with 1-alkanols with varying chain length *n*.
